# Supplementary material for: Electronics with correlated oxides: SrVO$_3$/SrTiO$_3$ as a Mott transistor
Source: arXiv:1312.5989 source file (2013-12-20)
Supplement: Supplementary file 1 [file DMFT_SVO_supplements_final.pdf]

# Supplementary Material of
# "Electronics with correlated oxides: $SrVO_3/SrTiO_3$ as a Mott transistor"

Zhicheng Zhong[1], Markus Wallerberger[1], Jan M. Tomczak[1], Ciro Taranto[1],
Nicolaus Parragh[2], Alessandro Toschi[1], Giorgio Sangiovanni[2], and Karsten Held[1]
[1] Institute of Solid State Physics, Vienna University of Technology, A-1040 Vienna, Austria
[2] Universität Würzburg, Am Hubland, D-97074 Würzburg, Germany

PACS numbers: 71.27.+a, 71.30.+h, 73.40.-c

## Correlation-induced crystal field splitting

The results presented in this Letter were obtained by combining density functional theory (DFT) and dynamical mean field theory (DMFT). DMFT corresponds to a mean field in space but allows for a dynamical description of local quantum fluctuations. As a consequence, the self-energy $\Sigma(k,\omega)$ is flat in $k$-space but, unlike LDA+U, still carries a frequency dependence: $\Sigma(k,\omega) = \Sigma(\omega)$. As solver for the auxiliary impurity problem of DMFT we used continuous-time quantum Monte Carlo (CTQMC) in the hybridization-expansion version. For more details about CTQMC and about our implementation see Refs. [1–3]. CTQMC is formulated in imaginary time and therefore uses Matsubara frequencies $\mathrm{i}\omega_n$. To obtain the corresponding real-axis quantity from $\Sigma(\mathrm{i}\omega_n)$ a Wick rotation is necessary. Two special limits of the self-energy are however readily interpretable on the Matsubara axis: The asymptotic behavior $\Sigma(\mathrm{i}\omega_n \to \infty)$ and the extrapolation $\Sigma(\mathrm{i}\omega_n \to 0)$.

In the following we discuss the self-energy and the enhanced orbital splitting derived from its real part extrapolated at zero frequency. The left panel of Fig. 1 shows the real part of the self-energies for different orbitals (colors), layers (point filling) and interaction strengths (point shapes) on the Matsubara axis $\mathrm{Re}\,\Sigma(\mathrm{i}\omega_n)$. The asymptotic constant $\mathrm{Re}\,\Sigma(\mathrm{i}\omega_n \to \infty)$ indicates the Hartree contributions to the electronic self-energy that depend in turn on the individual orbital occupations. The value $\mathrm{Re}\,\Sigma(\mathrm{i}\omega_n \to 0) = \mathrm{Re}\,\Sigma(\omega \to 0)$, or more precisely its difference between different orbitals, gives the many-body correction to the crystal field splitting. At the surface, the LDA crystal field splitting between the $xy$ and the $xz/yz$ orbital is enhanced by correlations in agreement with the general DMFT trend away from half-filling, see Ref. [4]. In the right panel of Fig. 1 one can also see how, close to $U' = 3.5\,\mathrm{eV}$, the crystal field rapidly changes at the metal-insulator transition.

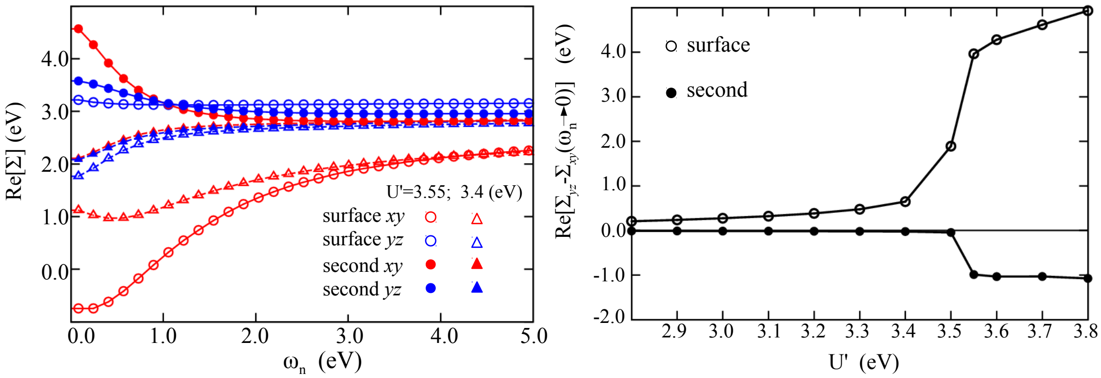


FIG. 1: Left panel: Real part of the self energies in Matsubara frequency for $U'$=3.55eV (3.4eV) with an insulating (metallic) state. The surface layer is denoted by unfilled circles (triangles), and the second layer is denoted by filled circles (triangles). $xy$ is in red, and $yz$ is in blue. Right panel: correlation-induced effective crystal field splitting as a function of $U'$. The crystal field splitting is defined as real part of self energy difference between $yz$ and $xy$ orbitals in the low frequency region. The surface layer is indicated by unfilled circle and the second layer is noted by filled circle.

## Coulomb interaction matrix elements

Besides the one-particle dispersion, also the Coulomb interaction matrix elements, needed for the LDA+DMFT calculations, are affected by the film and surface geometry. Here, we employ the constrained random phase approximation (cRPA)[5] within the setup of maximally localized Wannier functions[6, 7] to compute the on-site (local) elements of the Hubbard $U$. Owing to the prohibitive computational cost, we need to neglect the substrate and consider free-standing layers that are separated by at least 10Å of vacuum. However, we use the lattice constants and optimized internal positions as described in the manuscript. The Brillouin zone is discretized into a mesh of 8×8×8, 8×8×1 and 6×6×1 for the bulk, one-, two-layer, and three-layer setup, respectively. For further technical details see Ref. 7.

The left panel of Fig. 2 shows the diagonal elements of the bare on-site Coulomb interaction $V$ in the maximally localized Wannier function basis of the $t_{2g}$ subspace. The variation of the overall values solely stems from the different (real-space) extension and symmetry of the Wannier functions (see e.g. Ref. 8 for a discussion). Moreover, the breaking of translational invariance causes a lifting of the degeneracy between orbitals that have or have not lobes in the $z$ direction, which is the stacking order of the layers. Indeed, the $xy$ in-plane elements are close to the bulk value, whereas the $xz/yz$ components are smaller for the films, since the respective Wannier functions are more extended. This owes to the decreased coordination of the respective vanadium sites: there is less freedom to localize the orbitals by admixtures from neighboring atomic sites[8]. Naturally, this effect is particularly strong for the single layer. Already for three layers, the inner layer almost recovers the three-fold $t_{2g}$ degeneracy and has a bare $V$ and thus Wannier functions that are similar to the bulk.

For use in the effective $t_{2g}$ setup of the LDA+DMFT, the interaction is screened by the (here: RPA) polarization made up from all but the intra-$t_{2g}$ transitions. From the right panel of Fig. 2 we see that the smaller-than-bulk values for $V$ of the finite films are overcompensated by the difference in screening: The Hubbard $U$ for the films are larger than for the bulk, but approach the latter with growing number of layers. The $xy$ in-plane component is always larger than the $xz/yz$. As for the bare interaction, they are almost the same for the inner layer of the three-layers film. The relative orbital differentiation already seen in the bare interaction is not much affected by the screening. Therefore, the lifting of the degeneracy of the $U$ values can be mostly ascribed to the different extension of the Wannier functions.

The values of the Hubbard $U$ are on average enhanced by $\sim$ 20% ($\sim$ 10%) when going from the bulk to the mono-layer (bi-layer). A similar enhancement is found for the screened intra-orbital interaction $U'$. Let us note that the values are stronger enhanced for the $xy$ orbital that is found to be Mott-Hubbard insulating on the surface of the bi-layer film within our LDA+DMFT calculations. While this, and the spatial gradient of $U$ in the z-direction can be argued to cause a slight charge transfer towards the interface and into the degenerate $xz/yz$ orbitals, we do not expect a qualitative change in our physical picture. On the quantitative level, this may however influence the temperature at which the two-layers system exhibits an insulator-to-metal transition upon cooling. Yet, one has to

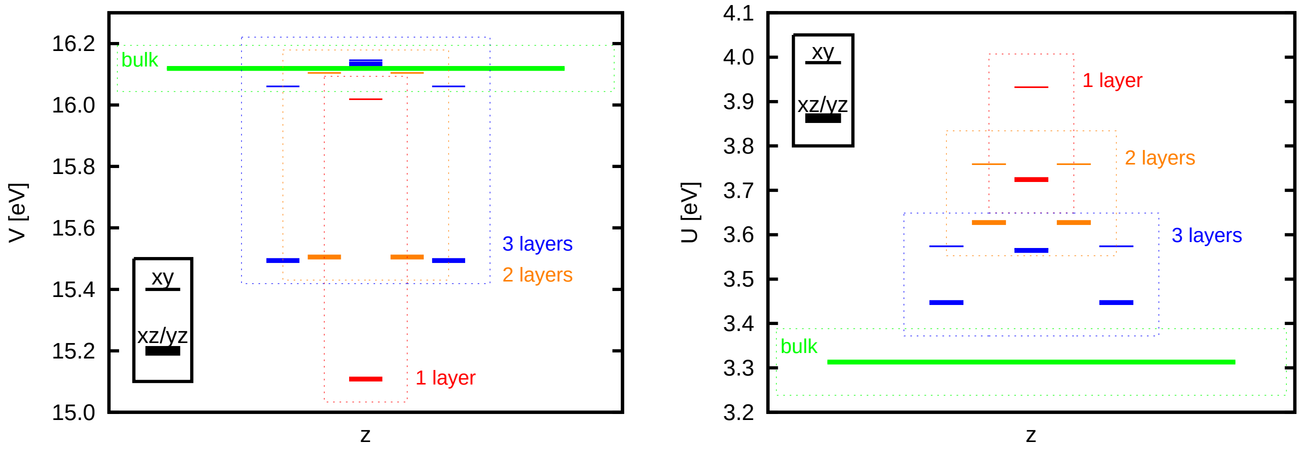


FIG. 2: Coulomb interaction matrix elements. Shown are the on-site and orbital diagonal (density-density) matrix elements of the Coulomb interaction in the maximally localized $t_{2g}$ Wannier function basis, resolved into $xy$ and $xz/yz$ orbitals and for one, two and three free-standing layers, as well as for bulk $SrVO_3$. Left panel: the bare/unscreened Coulomb interaction $V$; right panel: the partially screened, static intra-orbital Hubbard interaction $U$. The abscissa mimics the extension of the geometry in the $z$-direction.

keep in mind that the setup used for the computation of the interaction strengths, here, has been performed (owing to the computational cost) for free-standing films. In the real system the substrate on one side of the film will provide further screening channels, as well as variational freedom to localize the Wannier functions. Both effects decrease $U$ further toward the bulk value and reduce the layer and orbital differentiation in $V$ (and hence $U$). Roughly, we can argue that the enhancement and orbital differentiation seen here will be only half as strong for the setup used in the DFT+DMFT, since only one side of the films is exposed to vacuum.

## Surface effect on photoemission spectroscopy

We use four layers of $SrVO_3$ thin films grown on $SrTiO_3$ to simulate the surface effect, see Fig. 3 left panel. As for the two layer case, we find that the spectra of the topmost (surface) layer is very different from that of the other layers. The surface layer exhibits stronger correlation effects with an enhanced lower Hubbard band which is shifted by 0.5eV towards the Fermi level, while the other layers are more similar to the bulk spectrum. This is very similar to the two layer case in the main paper.

Photoemission spectroscopy (PES) is a surface sensitive technique. In the simplest approximation it yields an averaged spectrum with bulk weight rediuced $e^{-d/\lambda}$ and surface weightd $1 - e^{-d/\lambda}$ ($d$: $z$-axis lattice constant; $\lambda$: electron escape depth). In Fig. 3 we have taken the experimental penetration depths for two photon different energies, for details see Ref.[9]. As clearly shown in Fig. 3, including surface effect will give a better agreement with experiment. Let us cautiously remark though that our DFT+DMFT calculation was with a $SrTiO_3$ substrate since we were interested in the heterostructure, whereas the experiment was for the surface of pure $SrVO_3$ [9]. The qualitative effect should however be the same. Our finding is supported by very recent resonant soft-X-ray emission experiments [10].

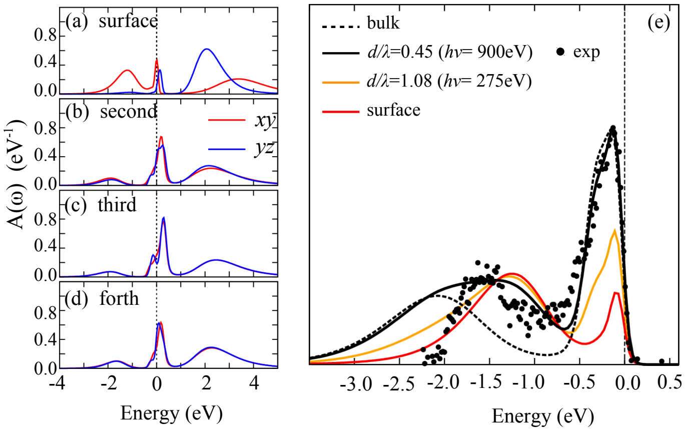


FIG. 3: Left: Spectra of four layers of $SrVO_3$ thin films grown on $SrTiO_3$. Right: Experimental photoemission [9] and theoretical bulk, surface, and simulated photoemission spectra of $SrVO_3$ for two different electron escape depths $\lambda$ (corresponding to two different photon energies $h\nu$).


[1] N. Parragh, Ph.D. Thesis, Universität Würzburg (2013).
[2] E. Gull, A. J. Millis, A. I. Lichtenstein, A. N. Rubtsov, M. Troyer, and P. Werner, Rev. Mod. Phys. **83**, 349 (2011).
[3] N. Parragh, A. Toschi, K. Held, and G. Sangiovanni, Phys. Rev. B **86**, 155158 (2012).
[4] N. Parragh, G. Sangiovanni, P. Hansmann, S. Hummel, K. Held, and A. Toschi, Phys. Rev. B **88**, 195116 (2013).
[5] F. Aryasetiawan, M. Imada, A. Georges et al., Phys. Rev. B **70**, 195104 (2004).
[6] N. Marzari and D. Vanderbilt, Phys. Rev. B **56**, 12847 (1997).
[7] T. Miyake and F. Aryasetiawan, Phys. Rev. B **77**, 085122 (2008).
[8] J. M. Tomczak, T. Miyake, R. Sakuma et al., Phys. Rev. B **79**, 235133 (2009).
[9] A. Sekiyama, H. Fujiwara, S. Imada, S. Suga, H. Eisaki, S. I. Uchida, K. Takegahara, H. Harima, Y. Saitoh, I. A. Nekrasov et al., Phys. Rev. Lett. **93**, 156402 (2004).
[10] J. Laverock, B. Chen, K. E. Smith, R. P. Singh, G. Balakrishnan, M. Gu, J. W. Lu, S. A. Wolf, R. M. Qiao, W. Yang, et al., Phys. Rev. Lett. **111**, 047402 (2013).
